# Supplementary material for: Saliency Can Be All You Need In Contrastive Self-Supervised Learning
Source: arXiv:2210.16776 source file (2022-10-30)
Supplement: Supplementary file 1 [file appendix.tex]

\section{Appendix}
\setcounter{table}{0}
\setcounter{figure}{0}

\subsection{Additional Experiments}
